# Supplementary material for: Mapping oil palm density at country scale: An active learning approach
Source: arXiv:2105.11207 source file (2021-05-24)
Supplement: Supplementary file 1 [file supplementary.tex]

\section{Supplementary}
\label{sec:suppl}

\input{algorithm_1}
